# Supplementary material for: Observation of tunable mobility edges in generalized Aubry-Andr\'{e} lattices
Source: arXiv:2007.01393 ancillary file (2020-07-02)
Supplement: Supplementary file 1 [file GAA_paper____supp.pdf]

# Supplementary Materials for: Observation of tunable mobility edges in generalized Aubry-André lattices

Fangzhao Alex An,[1,*] Karmela Padavić,[1,*] Eric J. Meier,[1] Suraj Hegde,[2] Sriram Ganeshan,[3,4,†] J. H. Pixley,[5,‡] Smitha Vishveshwara,[1,§] and Bryce Gadway[1,¶]

[1]*Department of Physics, University of Illinois at Urbana-Champaign, Urbana, IL 61801-3080, USA*
[2]*Max-Planck Institute for Physics of Complex Systems, 01187 Dresden, Germany*
[3]*Physics Department, City College of the CUNY, New York, NY 10031*
[4]*CUNY Graduate Center, New York, NY 10031*
[5]*Department of Physics and Astronomy, Center for Materials Theory, Rutgers University, Piscataway, NJ 08854 USA*
(Dated: July 2, 2020)

### Determination of the critical $\Delta/J$ values

For both experimental localization data and numerical simulations, we perform estimates for the "critical" value of the quasiperiodicity strength-to-tunneling strength ratio ($\Delta/J$) at which the localization transition occurs for each $\alpha$ value. These estimations are what contribute to the experimental data and lines in Fig. 3 of the main text (which are derived from Fig. S1(a,b)). A similar determination defines the solid lines appearing in Fig. S3, which reflect the expected localization transition for the lowest energy state (GS) and highest energy state (ES) in the presence of interactions.

To estimate the $\Delta/J$ transition values, we rely on a simple but robust determination that involves no fitting. For each $\alpha$ value and for a given state (ES or GS), we find where the normalized participation ratio (PR$/N$) crosses a threshold value $\mathrm{PR}_{\mathrm{thres}}/N = 0.19$. Specifically, for each $\alpha$ and for the GS or ES, we take a pairwise moving average to smooth out more jagged sections of the data, we perform a linear interpolation between the points, and we determine the $\Delta/J$ value at which the interpolated curve crosses $\mathrm{PR}_{\mathrm{thres}}$. This crossing value defines the localization boundaries appearing in, *e.g.*, Fig. 3 of the main text. We note that the exact value of $\mathrm{PR}_{\mathrm{thres}}/N = 0.19$ is simply chosen to provide a robust determination transition points, the results of which can be equally compared between experiment and simulation.

### Experimental localization transition lines

Figure 3 of the main text displays localization transition lines determined from the data according to the procedure outlined in the previous section. Here, we present the data sets for the GS and ES from which these localization curves were derived. In Fig. S1, we plot the measured PR$/N$ values for the GS and ES as prepared in experiment, as a function of the quasiperiodicity strength-to-tunneling strength ratio $\Delta/J$ and the GAA tuning parameter $\alpha$. The state preparation ramp is the same as described for Fig. 2 of the main text. The black line-connected data points in Fig. S1 panels (a) and (b) denote critical $\Delta/J$ values for the GS and ES, respectively. These are determined for each $\alpha$ column by finding where the measured PR$/N$ exceeds the threshold value of 0.19. Shifts in the delocalization transition for these two states show opposite trends: the GS transition shifts to larger $\Delta/J$ values for increasing $\alpha$, whereas the ES transition shifts to smaller $\Delta/J$ values for increasing $\alpha$. These trends are consistent with the simple single-particle picture outlined in the main text. Additional interaction effects further modify this picture, as discussed in the main text and below.

### Details of interactions in momentum space

This work is based on synthetic lattices of atomic momentum modes, populated by the atoms from a Bose-Einstein condensate of $^{87}$Rb. The ultracold neutral atoms are well-described as having $s$-wave contact interactions, which stem from Van der Waals interactions. In momentum-space, these interactions are long-ranged, such that atoms in any given momentum mode will interact with atoms from all of the various other modes. When all atoms occupy the zero-momentum condensate, there is a collective interaction energy shift $U$ per atom, relating to the chemical potential of the condensate.

Intra-mode collisions between the atoms are independent of the mode's momentum. For a pair of atoms colliding with a relatively low center-of-mass collision energy (below $\sim k_B \times 100\mu$K, with $k_B$ the Boltzmann constant), the collision strength should naively be the same for any modal combination (*i.e.*, for all intra- and inter-mode collisions), as summarized by Eq. (4) of the main text. However, the atoms populating the system are identical scalar bosons, so an effective mode-dependence arises due to quantum statistics. If $u = U/N_{\mathrm{at}}$ represents the pairwise interaction energy for two atoms "colliding" in the same momentum mode through direct interactions, then a pair of identical bosons occupying distinct modes experience twice that interaction energy $2u$ because of exchange interactions [1].

Interactions between atoms in the synthetic lattice then have a peculiar form – long-ranged and all-to-all,

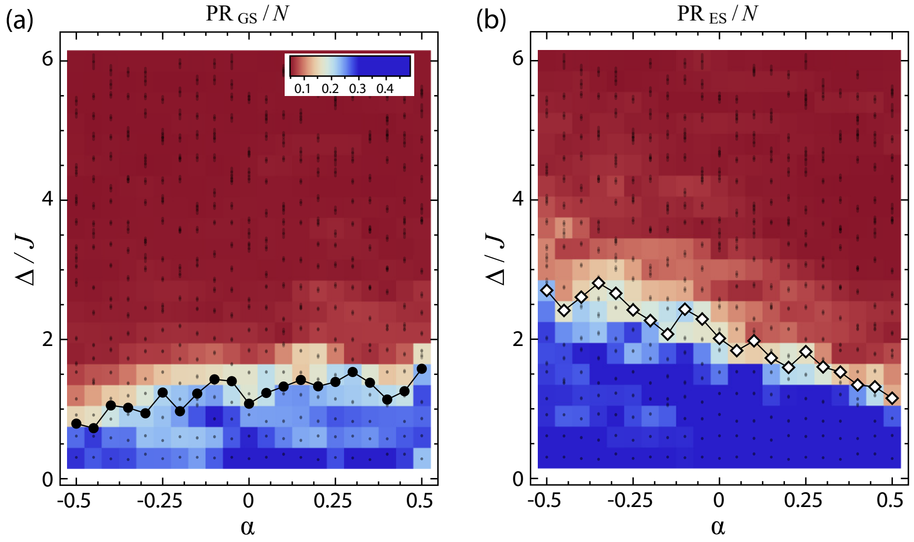


FIG. S1. **Localization phase diagram of the GS and ES. (a,b)** The localization phase diagrams of PR/$N$ vs. $\Delta/J$ and $\alpha$ for the (a) ground state (GS) and (b) highest excited state (ES). Filled circles and open diamonds mark the "critical" $\Delta/J$ for each $\alpha$ value, calculated by determining where the PR/$N$ dips below a threshold $\mathrm{PR}_{\mathrm{thres}}/N = 0.19$. The PR is plotted according to the inset color bar, based on data sampled at parameter values corresponding to the overlaid black points. Data points above $\Delta/J > 6$ are omitted for clarity.

but with a strength that is twice as large for inter-mode collisions than for intra-mode collisions. For the positive scattering length $a \approx 100\, a_0$ of our $^{87}$Rb atoms (repulsive real space interactions) these interactions shift the chemical potential for various synthetic lattice "sites" based on the modal populations. To illustrate this interaction shift, we consider the situation in which all population resides at a central lattice site (momentum order). The central site's chemical potential is shifted up by a collective energy $U$, while all other sites are shifted up by an energy of approximately $2U$. We subtract off a total shift of $2U$ from the interaction energy per particle to obtain a more intuitive *site-local* form of interactions. This effectively removes the off-site contributions, and leaves only a site-local *attraction* at the initially populated mode with a chemical potential shift of $-U$.

This discussion is essentially equivalent to taking the difference between the Bogoliubov spectrum and the single-particle spectrum for the system, sampled at a discrete set of momentum values, and introducing an offset of $2U$. We note that we ignore corrections due to superfluid screening, which in the above example leads to slightly smaller chemical potential shifts ($< 2U$) for the sites nearest to the condensate mode (because they are not entirely distinct from the condensate).

Throughout this section, our discussion of interactions has assumed a mean-field picture. As noted in the main text, our theoretical treatment is also at the mean-field level. Specifically, we describe the atomic population by a normalized complex wave function $\psi$ that solves the Gross-Pitaevskii equation (GPE) (non-linear Schrödinger equation). This approach ignores quantum fluctuations of the atomic distribution. Given the number of atoms in the experiment ($N_{\mathrm{at}} \sim 10^5$) and the length of the synthetic lattice ($N = 21$), this approximation is fairly well justified. Concretely, for a given occupied momentum order, we have $|\langle c_i \rangle| \approx |\langle c_i^\dagger \rangle| \approx |\psi_i| \times N_{\mathrm{at}} \gg 1$. We also expect any non-classical effects resulting from interactions to be beyond the ability of our current experimental probes. With these considerations, we find that the simple mean-field treatment captures most of the salient features of our experimental results.

We make two further simplifying assumptions concerning experimental details of atomic interactions and assume that (1) the atomic density and scale for $U$ are fixed in time, and that (2) $U$ is a homogeneous mean-field energy. A more precise analysis would consider the spatial variation of $\rho$, and thus $U$, across the trapped atomic sample and their dynamical response to the ramp in system parameters. We find that even without this more precise treatment there is good agreement between experiment and the GPE simulations.

Finally, we have thus far only discussed "diagonal" collisions that preserve the atomic populations of the colliding modes. In reality, a full continuum of momenta may be populated through collisions. However, mode-changing collisions are suppressed relative to mode-conserving ones, with our experiments operating in a regime in which the inelastic scattering rate is smaller than the forward scattering rate. Thus we make the simplifying assumption that all collisions are mode-conserving, and ignore all collisional scattering out of our defined lattice of momentum modes.

### Numerical treatment of interactions

We perform three types of numerical simulations in this work: (1) exact diagonalization of the tight-binding GAA Hamiltonian, (2) simulations of the time-dependent GPE having an attractive Hartree interaction term, and (3) imaginary time propagation calculations determining GPE ground and excited state wavefunctions, respectively, in the presence of such interactions.

Our GPE simulations follow from arguments outlined in the previous section. Namely, since the typical occupation of the coupled momentum modes in our experiment is large, we describe the atom population with a normalized complex wave function $\psi$ that solves the GPE and include a mean-field interaction term (or Hartree term) as $-U|\psi|^2\psi$. Dynamical simulations that incorporate the experimental parameter ramp procedure, as appearing in the main text Fig. 2, are performed by evolving this nonlinear Schrödinger equation, with inclusion of the $-U|\psi|^2\psi$ term.

Alternatively, we can also compare to the true eigenstates of the interacting GAA model, determined via imaginary time propagation of the same GPE with mean-field interactions. Here, we substitute imaginary time $\tau = \pm it$ for the real time $t$ in the time-dependent nonlinear Schrödinger equation and evolve to find the ES and the GS, respectively. The wave-function obtained in this way approximates either the lowest (GS) or highest (ES) energy state of the system as all other contributions decay exponentially. Our imaginary time-propagation calculations are iterative: the approximate GS (ES) state $\psi$, appropriately normalized, is used as a trial wavefunction in the next calculation. Typically, we perform 100 iterative loops, each having a 2 ms timescale.

Figure S2 summarizes the localization behavior of the exact eigenstates as determined by imaginary time propagation. Qualitatively, the same trends are observed as in Fig. 2(c) of the main text (which considered the time-evolved "ramping" results): a ME that is tuned by the parameter $\alpha$, with enhanced GS localization for $\alpha = -0.5$, enhanced ES localization for $\alpha = +0.5$, and the appearance of a ME at $\alpha = 0$ due to interactions. However, the PR/$N$ values show a distinct deviation from the time-evolved results of main text Fig. 2(c), particularly for $\alpha = -0.5$ and $\alpha = 0$. As discussed below, this discrepancy between the behavior of the true ES and the prepared state is a consequence of the ramping procedure and screening effects.

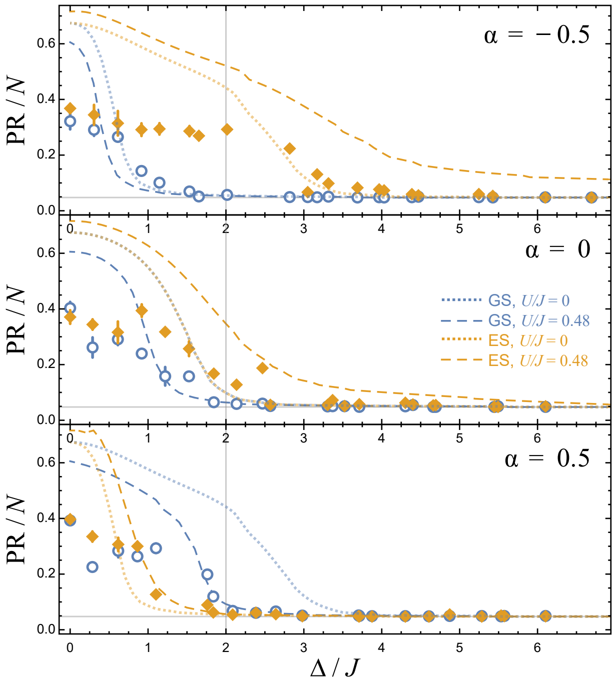


FIG. S2. **Localization behavior vs. the quasiperiodicity-to-tunneling strength ratio of the true GS and ES.** PR/$N$ vs. $\Delta/J$ for the ground (GS, open blue circles) and highest excited states (ES, yellow diamonds) under $\alpha = -0.5, 0, 0.5$, showing evidence for a mobility edge tunable via $\alpha$. The blue and yellow curves respectively relate to the true GS and ES of the system (*i.e.*, as determined by imaginary time propagation, ignoring effects due to the experimental preparation protocol). Long-dashed curves assume a homogeneous mean-field energy $U = 0.48J$, while short-dashed curves correspond to $U = 0$.

### Interaction effects on experimental state preparation

From Fig. S2, it is evident that for $\alpha \leq 0$, experimental ES data deviates from results of imaginary time-propagation calculations, as the latter indicate relatively higher PR/$N$ values. We attribute this discrepancy to interaction effects, namely screening by attractive interactions, and the details of the ramp procedure. Figure 1(a) of the main text illustrates that for $\alpha < 0$ there are many lattice sites lying at high energy. The effectively attractive interactions can serve to screen the quasiperiodic potential for the high energy states. This results in the ES being localized and restricted to the highest energy sites for large $\Delta/J$, but still populating multiple high energy sites whose site energy differences fulfill $\Delta\epsilon \lesssim U$.

In experiment, we initialize population on only one lattice site and ramp the tunneling from zero to a final strength $J$. As the quasiperiodicity amplitude $\Delta$ is fixed for each ramp, this effectively ramps from the limit $\Delta/J = \infty$, where all eigenstates are site-localized in the absence of interactions, to some final $\Delta/J$ value. However, the existence of a fixed interaction strength $U$ throughout the ramp, and thus a non-zero $U/\Delta$, prohibits us from preparing the true highest energy eigenstate. A more ideal ramp procedure would lower both $\Delta/J$ and $\Delta/U$ from the infinite quasiperiodicity limit, to account for the fact that population needs to spread from the initial single site due to screening. We note that our

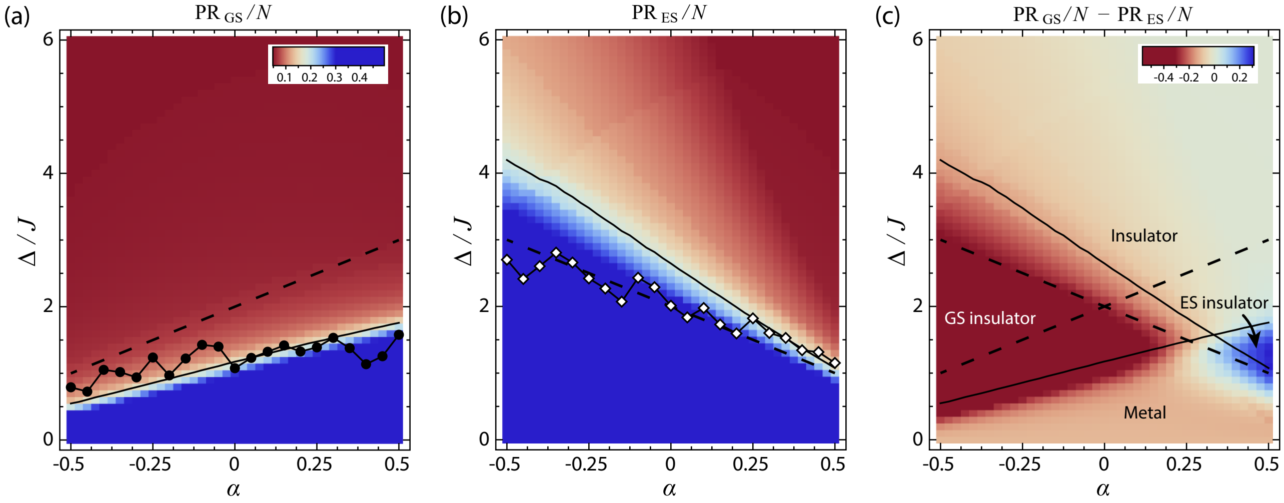


FIG. S3. **Numerical simulations of GS and ES localization phase diagrams.** The color in (a,b) represents PR/$N$ of the interacting eigenstates calculated by imaginary time propagation. The line-connected black circles and white in (a) and (b) are the transition curves found for the GS and ES from experiment, as in Fig. S1 and main text Fig. 3. Dashed lines represent the non-interacting transition lines determined based on the ME relation. Solid lines represent the critical $\Delta/J$ transition values, as determined for the interacting eigenstates (for $U = 0.48J$) by determining where PR/$N$ crosses the threshold value of 0.19. (c) The color shows the difference in the PR/$N$ for the GS and ES with interactions. Overlaid on this PR difference diagram are the theoretical critical delocalization boundaries, from (a) and (b).

ramping procedure is not a problem for the ground state preparation, as the effectively attractive interactions promote self-trapping for low-energy states.

### Localization trends in the presence of interactions

Figure S3 shows the numerically-calculated (by imaginary time propagation) localization phase diagrams for the eigenstates of the interacting GAA model, assuming a homogeneous mean-field interaction energy $U = 0.48J$. Along with the simulation results, we show experimental transition curves as in Fig. S1 for comparison (circles and diamonds indicate critical $\Delta/J$ values for the GS and ES, respectively). The background color in Figure S3 (a,b) represent the PR/$N$ for the GS and ES. Dashed lines indicate the expected $U = 0$ transition lines of $(\Delta/J)_c = 2(1 \pm \alpha)$ for the GS/ES, anticipated based on the GAA ME relation given in Eq. (3) of the main text. Solid lines show critical $\Delta/J$ values for the *interacting* eigenstates (calculated by imaginary time propagation), determined by comparison to a threshold value of PR/$N$. The discrepancy between the dashed (non-interacting) and solid (interacting) lines underscores the shifting of the ME due to interactions.

As the experimental data for the GS agrees with the interacting theory curves, we conclude that we see clear effects of self-trapping in experiment. In contrast, for the ES (in particular for $\alpha \lesssim 0$), our experimental results align more with the expected non-interacting transition curve than the one incorporating screening effects. This signifies that our state preparation procedure was likely unable to capture the exact behavior of the true ES across the full parameter space, due to our initial conditions and the effects of screening on the true ES.

* These authors contributed equally to this work.
† sganeshan@ccny.cuny.edu
‡ jed.pixley@physics.rutgers.edu
§ smivish@illinois.edu
¶ bgadway@illinois.edu

[1] R. Ozeri, N. Katz, J. Steinhauer, and N. Davidson, Rev. Mod. Phys. **77**, 187 (2005).
